# Supplementary material for: A unified, geometric framework for nonequilibrium protocol optimization
Source: arXiv:2205.01205 source file (2022-12-05)
Supplement: Supplementary file 1 [file appendix_spl.tex]

\documentclass[%
superscriptaddress,
notitlepage,
groupedaddress,
amsmath,amssymb,
aps,
floatfix,
]{revtex4-2}

\usepackage{graphicx}% Include figure files
\usepackage{dcolumn}% Align table columns on decimal point
\usepackage{bm}% bold math

%%% HELPER CODE FOR DEALING WITH EXTERNAL REFERENCES
\usepackage{xr-hyper}
\makeatletter
\newcommand*{\addFileDependency}[1]{
  \typeout{(#1)}
  \@addtofilelist{#1}
  \IfFileExists{#1}{}{\typeout{No file #1.}}
}
\makeatother

\newcommand*{\myexternaldocument}[1]{
    \externaldocument{#1}
    \addFileDependency{#1.tex}
    \addFileDependency{#1.aux}
}
%%% END HELPER CODE

% put all the external documents here!

\myexternaldocument{main}

\input{preamble}

\begin{document}
\title{Unifying thermodynamic geometries}

\author{Shriram Chennakesavalu}
\email{shriramc@stanford.edu}
\affiliation{Department of Chemistry, Stanford University, Stanford, CA 94305}%
\author{Grant M. Rotskoff}%
 \email{rotskoff@stanford.edu}
\affiliation{Department of Chemistry, Stanford University, Stanford, CA 94305}%

\date{\today}% It is always \today, today,
             %  but any date may be explicitly specified

\maketitle

\input{appendix}

\newpage
\bibliography{refs_app}

\end{document}
